# Supplementary material for: Learning to Compose Domain-Specific Transformations for Data Augmentation
Source: arXiv:1709.01643 source file (2017-09-30)
Supplement: Supplementary file 1 [file tanda_appendix.tex]

\subsection{Synthetic Data Example}

\begin{figure}
\centering
\begin{subfigure}{.33\textwidth}
  \centering
  \includegraphics[width=1.0\linewidth]{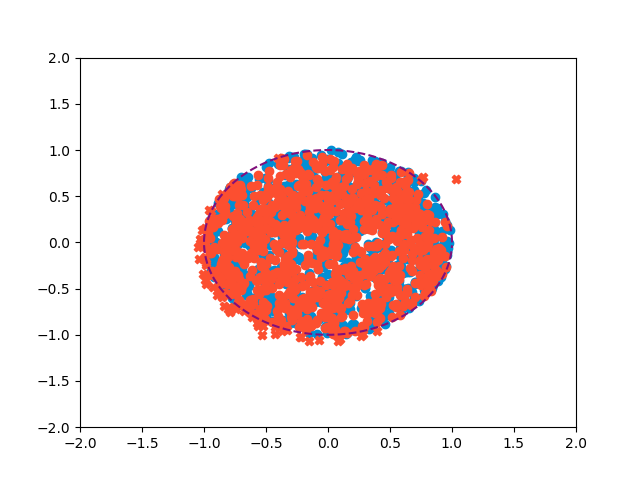}
  \caption{Mean field model on TF set 1}
  \label{fig:sub1}
\end{subfigure}%
\begin{subfigure}{.33\textwidth}
  \centering
  \includegraphics[width=1.0\linewidth]{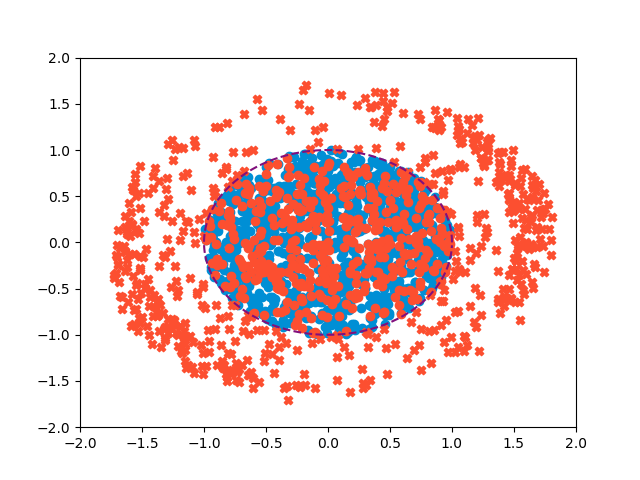}
  \caption{Mean field model on TF set 2}
  \label{fig:sub2}
\end{subfigure}
\begin{subfigure}{.33\textwidth}
  \centering
  \includegraphics[width=1.0\linewidth]{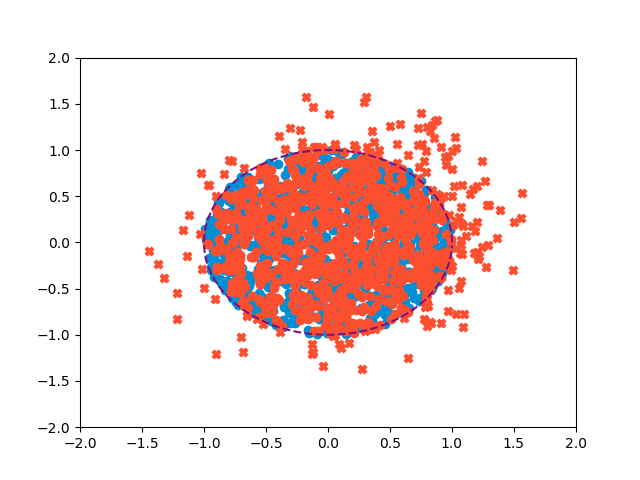}
  \caption{LSTM model on TF set 2}
  \label{fig:sub3}
\end{subfigure}
\caption{Original data points (blue) are transformed using sequences of vector displacement TFs ($L=10$) drawn from $G_\theta$, producing augmented data points (red). $G_\theta$ is either a mean field model or an LSTM, trained with an orcale discriminator $D^\emptyset$ for 15 epochs.}
\label{synthetics}
\end{figure}

As a simple example, we consider a set of points uniformly distributed in the unit ball around the origin.
In this setting, we define $y_\emptyset (x) = 1\{ ||x|| \ge 1 \}$, and consider two different TF sets:
\begin{compactenum}
\item \textit{Good vs. Bad TFs:}
In a first toy scenario we consider TFs which are vector displacements of random direction, with magnitude drawn from one of two distributions, $\mathcal{N}(\mu_1, \sigma_1)$ or $\mathcal{N}(\mu_2, \sigma_2)$, where $\mu_1 > 1 > \mu_2$.
In other words, the model should learn not to select certain individual TFs.

\item \textit{Lossy TFs:}
We consider a second toy setting where random-direction displacement TFs have magnitude drawn uniformly from $\mathcal{N}(\mu, \sigma)$, $\mu < 1$; however the magnitude of each TF decays exponentially with the distance a point is outside of the unit ball.
This simulates the setting where TFs are irrecoverably lossy when applied in certain sequences.
\end{compactenum}
As expected, we see that while the mean field model is able to model the first setting (Figure~\ref{fig:sub1}), it fails to adequately represent the second one (Figure~\ref{fig:sub2}), whereas the RNN model is able to (Figure~\ref{fig:sub3}).

%%% Effects of Sequence Length and Diversity Term
\subsection{Sensitivity to Sequence Length and Diversity Term}
\label{subsec:sensitivity}
The length of the transformation sequence and the strength of the diversity objective term are two critical hyperparameters of the generative model, and we seek to quantify TANDA's sensitivity to their values.
We trained a set of generative models on CIFAR10, varying only the sequence length, and used these to train end classifiers.
The procedure was repeated, but varying only the coefficient of the pixel distance term.
\ajr{TODO: Run and plot this experiment!}

%%% Coverage and Class Invariance
% - An analysis by nearest neighbor proxy of (a) coverage and (b) class invariance
\subsection{Coverage of the input space}
\label{subsec:coverage}

In Section %\ref{sec:x}
, we motivated the use of the two objective terms for the generative model.
While the discriminative loss term encourages the generator to produce transformed images that fall within the underlying (unlabeled) data distribution, the diversity term encourages increased coverage of the input space.
As a visual proxy, Figure \ref{fig:coverage} shows examples of MNIST images transformed using both TANDA and random sequences of transformations.
We also show the closest images in the entire MNIST dataset by pixel distance.
While random transformations are at risk of entering the null class or not improve coverage near unseen examples, the TANDA-transformed images demonstrate class invariance while moving away from their class' center-of-mass.

\begin{figure}
\centering
\begin{subfigure}{.45\textwidth}
  \centering
  \includegraphics[width=1.0\linewidth]{figs/tanda-nn_1}
  \caption{}
  \label{fig:coverage-1}
\end{subfigure}\hfill
\begin{subfigure}{.45\textwidth}
  \centering
  \includegraphics[width=1.0\linewidth]{figs/tanda-nn_2}
  \caption{}
  \label{fig:coverage-2}
\end{subfigure}
\caption{Randomly selected images of a ``4'' and a ``6'', transformed using TANDA (LSTM) and at random.
A sequence length of 10 was used.
In Figure \ref{fig:coverage-1}, the randomly transformed image entered the null class, while the TANDA image did not.
In Figure \ref{fig:coverage-2}, the TANDA image appears to be close to the decision boundary.}
\label{fig:coverage}
\end{figure}

In Table \ref{tab:coverage}, we compute summary statistics over the entire MNIST dataset.
\hank{Analysis of statistics.}

\begin{table*}[htbp!]
\centering
\setlength\tabcolsep{5pt} 
\begin{tabular}{lcc}
\toprule
 & {\bf \small \% of neighbors with different class} & {\bf \small Median \# of unique classes in neighborhood}\\
\midrule 
TANDA & &  \\
Random & &  \\
\bottomrule 
\end{tabular}
\caption{Statistics for pixel-distance neighborhoods (10 closest points) of transformed data points over the entire MNIST dataset.}
\label{tab:coverage}
\end{table*}

\subsection{Robustness to Transformations}
Supplementary data:
\begin{table*}[htbp!]
\centering
\setlength\tabcolsep{5pt} 
\small{
\begin{tabular}{ll|c|cccccccccc}
\toprule
 & & {\bf None} & \multicolumn{2}{c}{\bf Rotation} & \multicolumn{2}{c}{\bf Zoom} & \multicolumn{2}{c}{\bf Blur} & \multicolumn{2}{c}{\bf Shear} & \multicolumn{2}{c}{\bf Hue}\\
 & & & L & S & L & S & L & S & L & S & L & S \\
\midrule
CIFAR10 & {\it -} & 64.48 & 60.58 & 62.70 & 59.15 & 61.53 & 64.48 & 64.48 & 60.28 & 63.21 & 58.16 & 62.65 \\
 & {\it R} & 73.24 & 73.03 & 74.11 & 72.77 & 73.32 & 73.24 & 73.24 & 73.30 & 73.44 & 72.84 & 73.03 \\
 & {\it T} & 76.63 & 74.48 & 75.96 & 74.64 & 75.66 & 76.63 & 76.63 & 74.91 & 76.05 & 75.35 & 76.07 \\
\bottomrule 
\end{tabular}
}
\caption{Accuracy scores on random 10\% subsamples of test data (\textit{None}) and on versions augmented with a single transformation (\textit{Rotation}, etc.) with parameters drawn uniformly from large (\textit{L}) or small (\textit{S}) ranges; averaged over ten random subsamples / trials. \ajr{TODO: Change this into bar chart?}}
\end{table*}

\subsection{Basic policy gradient approach}
We can derive our gradient update, using the standard ``likelihood-ratio'' trick.
A common variance reduction technique is to replace the reward with the \textbf{advantage} $A(s) = R(s) - b(s)$, where $b(s)$ is a \textbf{baseline} term. This does not change the expected value of the gradient.
\begin{align*}
    \nabla_\theta U(\theta) &= \nabla_\theta E_{\tilde{X},\tau}\left[ A(s)\ | \ \pi_\theta \right]\\
    &= \nabla_\theta E_{\tilde{X}} \left[ \sum_\tau P(\tau; \theta)A(s) \right]\\
    &= E_{\tilde{X}} \left[ \sum_\tau \nabla_\theta P(\tau; \theta)A(s) \right]\\
    &= E_{\tilde{X}} \left[ \sum_\tau \frac{P(\tau; \theta)}{P(\tau; \theta)} \nabla_\theta P(\tau; \theta)A(s) \right]\\
    &= E_{\tilde{X}} \left[ \sum_\tau P(\tau; \theta) \nabla_\theta \log P(\tau; \theta)A(s) \right]\\
    &= E_{\tilde{X},\tau} \left[ \nabla_\theta \log P(\tau; \theta)A(s) \right]
\end{align*}
Factorizing the probability of the chain \textit{\'{a} la} recurrent policy gradients yields
\[\nabla_\theta U(\theta) = E_{\tilde{X},\tau} \left[A(s) \sum_{t=1}^T \nabla_\theta \log \pi_\theta(a_t\ |\ \hat{s}_{t-1}) \right]\]

We can then approximate via sampling (over a batch of $n$ data points and $m$ sampled action sequences per data point):
\begin{align*}
    \nabla_\theta U(\theta) &\approx \frac{1}{nm}\sum_{i=1}^n\sum_{j=1}^m  A(x^{(i)}, \tau^{(j)})\sum_{t=1}^T \nabla_\theta \log \pi_\theta(a^{(j)}_t\ |\ \hat{s}^{(i,j)}_{t-1})
\end{align*}

\subsection{Variance reduction methods}
We can reduce the variance even further using standard techniques.
One way is to use the fact that an action at time $t$ can only be rewarded for outcomes at times $t' \ge t$:
\begin{align*}
    \nabla_\theta U(\theta) &= \frac{1}{nm}\sum_{i=1}^n\sum_{j=1}^m \sum_{t=1}^T \nabla_\theta \log \pi_\theta(a_t^{(j)}\ |\ \hat{s}^{(i,j)}_{t-1}) \left(\sum_{t'=t}^T R(s^{(i,j)}_{t'}) - b(s_{t'})\right)\\ 
\end{align*}

We can use a simple baseline which is the expected current and future reward at time $t'$ across all chains and examples in the batch:
\begin{align*}
    b_{t} = E_{\tilde{X},\tau}\left[\sum_{t'=t}^T R(s_{t'})\right]
    \approx \frac{1}{nm}\sum_{i=1}^n\sum_{j=1}^m \sum_{t'=t}^T R(s^{(i,j)}_{t'})
    = \frac{1}{nm}\sum_{i=1}^n\sum_{j=1}^m \left(\ell_D(\tilde{x}^{(i,j)}_{t-1}) - \ell_D(\tilde{x}^{(i,j)})\right)
\end{align*}

Then the above gradient is given by
\begin{align*}
    \nabla_\theta U(\theta) &= \frac{1}{nm}\sum_{i=1}^n\sum_{j=1}^m \sum_{t=1}^T \nabla_\theta \log \pi_\theta(a_t^{(j)}\ |\ \hat{s}^{(i,j)}_{t-1}) \left(\left(\sum_{t'=t}^T R(\hat{s}^{(i,j)}_{t'})\right) - b_t\right)\\
    &=\frac{1}{nm}\sum_{i=1}^n\sum_{j=1}^m \sum_{t=1}^T \nabla_\theta \log \pi_\theta(a_t^{(j)}\ |\ \hat{s}^{(i,j)}_{t-1}) \left(\ell_D(\tilde{x}^{(i,j)}_{t-1}) - \ell_D(\tilde{x}^{(i,j)}) - b_t\right)
\end{align*}

\subsection{From Section 4}
\paragraph*{Reinforcement Learning Formulation}

%Given a sequence of $L$ transformation function indices $\tau=\left(\tau_1, ..., \tau_L\right)\sim G_{\theta}$ and a data point $x$, we produce a sequence of incrementally transformed data points $\left(x, \tilde{x}_1, ..., \tilde{x}_{L-1}, \tilde{x}_L\right)$.
%Ultimately, our goal is to augment the training dataset of an end discriminative model using only the final transformed point, $\tilde{x}_L$.
%However, we can utilize the whole sequence for training $G_\theta$.

Let $\tau_i$ be the index of the $i$th TF applied, and $\tilde{x}_i$ be the resulting incrementally-transformed data point. Then we consider $s_t = \left({x, \tilde{x}_1, \tilde{x}_2,..., \tilde{x}_t, \tau_1, ...., \tau_t}\right)$ as the state after having applied $t$ of the incremental TFs.
Note that we include the incrementally transformed data points $\tilde{x}_1, ..., \tilde{x}_t$ in $s_t$ since the TFs may be stochastic.
Each of the model classes considered for $G_\theta$ then utilizes a different \textit{state representation} $\hat{s}$.
For the mean field model, the state representation used is $\hat{s}_t^{\text{MF}} = \emptyset$.
For the LSTM model, we use $\hat{s}_t^{\text{LSTM}} = \textsf{LSTM}(\tau_t, s_{t-1})$, the state update operation performed by a standard LSTM cell parameterized by $\theta$.

\paragraph*{Policy Gradient with Incremental Rewards}
Let $\ell_t(x,\tau) = \log (1 -D_\phi^\emptyset(\tilde{x}_t) )$ be the \textit{cumulative loss} for a data point $x$ at time $t$, with $\ell_0(x) = \ell_0(x,\tau) \equiv \log (1-D_\phi^\emptyset(x))$, and let $R(s_t) = \ell_t(x,\tau) - \ell_{t-1}(x,\tau)$ be the \textit{incremental reward}.
We can now recast the first term of our objective $\tilde{O}_\emptyset$ as an expected sum of incremental rewards:
\begin{align*}
U(\theta) &\equiv \mathbb{E}_{\tau\sim G_{\theta}}
                \mathbb{E}_{x\sim\mathcal{U}}\left[ 
                    \log(1 - D_\phi^\emptyset(h_{\tau_1}\circ\hdots\circ h_{\tau_L}(x)))
                \right]
             = \mathbb{E}_{\tau\sim G_{\theta}}
                \mathbb{E}_{x\sim\mathcal{U}}\left[ 
                    \ell_0(x) + \sum_{t=1}^L R(s_t)
                \right]
\end{align*}
The incremental reward is simply the difference in discriminator loss at each incremental transformation step.
We omit $\ell_0$ in practice, equivalent to using the loss of $x$ as a baseline term.

Let $\pi_\theta$ be the stochastic transition policy implictly defined by $G_\theta$. We compute the recurrent policy gradient~\cite{wierstra2010recurrent} of the objective $U(\theta)$ as:
\begin{align*}
\nabla_\theta U(\theta) &= \mathbb{E}_{\tau\sim G_{\theta}}
                \mathbb{E}_{x\sim\mathcal{U}}\left[ 
                    \sum_{t=1}^L R(s_t) \nabla_\theta \log \pi_\theta(\tau_t\ |\ \hat{s}_{t-1})
                \right]
\end{align*}
We approximate this quantity by sampling batches of $n$ data points and $m$ sampled action sequences per data point.
In practice, we use standard techniques of discounting with factor $\gamma\in [0,1]$ and considering only future rewards~\cite{greensmith2004variance}:
\begin{align*}
    \nabla_\theta U(\theta) &\approx 
        \frac{1}{nm} \sum_{i=1}^n \sum_{j=1}^m 
            \sum_{t=1}^L \nabla_\theta \log \pi_\theta(\tau_t^{(j)}\ |\ \hat{s}^{(i,j)}_{t-1})
            \left(
                \left(
                    \sum_{t'=t}^L \gamma^{t'-t}R(\hat{s}^{(i,j)}_{t'})
                \right)
                - b(s_{t'})
            \right)
\end{align*}
where $b(s_{t'})$ is a Monte Carlo estimate of the discounted future rewards.

\subsection{Transformation Regularization Term}

Motivated by this potential for complimentary enhancement, we combine our approach with that of \cite{SajjadiJT16a} by adding a \textit{transformation robustness} term to our end classifier's loss function that encourages minimization of the divergence in predicted marginals between each \textit{unlabeled} datapoint $x\in\mathcal{U}$ and its transformed copy:
\begin{align*}
O_{tr} &= E_{\tau\sim G(\cdot;\:\theta)} \left[
                E_{x\sim\mathcal{U}}\left[ 
                    \|f_w(x) - f_w(h_{\tau_L}\circ\hdots\circ h_{\tau_1}(x))\|
                \right]
            \right]
\end{align*}
where $f_w$ is the final pre-softmax layer of $D^f_w$.
We note that this is also similar to the \textit{local distributional smoothness} term in \cite{miyato2015distributional}, except that we compare a point to a transformed copy produced by our approach, rather than computing an adversarially-perturbed version.
Whereas the latter approach adds computational cost, requiring three additional forward-backward propagation passes, ours adds no additional cost given our setup.
On CIFAR10, we see a \ajr{X\%} boost in sei-supervised accuracy using this addition.
By additionally adding in the other techniques utilized in \cite{SajjadiJT16a} (\ajr{...}), we get a \ajr{X\% boost over} their state-of-the-art semisupervised CIFAR10 score.
